# Supplementary material for: GenDeg: Diffusion-based Degradation Synthesis for Generalizable All-In-One Image Restoration
Source: arXiv:2411.17687 source file (2025-03-22)
Supplement: Supplementary file 1 [file X_suppl.tex]

\clearpage
\setcounter{page}{1}
\setcounter{equation}{0}
\setcounter{figure}{0}
\setcounter{table}{0}
\setcounter{section}{0}
\makeatletter

\makeatletter
\makeatother

% \nolinenumbers
\maketitlesupplementary

\section{Overview}
% FID for generated images
% User study
% 
In this supplementary, we begin by showcasing 
samples from the GenDS dataset along with dataset statistics, followed by comparing diffusion model conditioning with and without $\mu$ and $\sigma$. Next, we examine the influence of structure correction, $S$, on the quality of the generated images. We then provide more details about the dataset filtering strategy discussed in Sec.~\ref{subsec: synthdataset}, followed by examples showcasing the effect of $3\times 3$ convolutions in the decoder of the Swin-model for suppressing patch-border artifacts discussed in Sec.~\ref{subsec: genirmodel}. Subsequently, we provide implementation details and a comprehensive overview of the dataset used for training and out-of-distribution (OoD) testing. We then discuss related works on diffusion models and limitations of our method. Finally, we present detailed quantitative results and additional qualitative comparisons.

\noindent To summarize, the supplementary discusses the following:
\begin{enumerate} 

\item Samples from the GenDS dataset 

\item Conditioning with and without $\mu, \sigma$

\item Impact of structure correction $S$ 

\item Dataset filtering thresholds 

\item Comparison of 1x1 and 3x3 convolutions in the Swin decoder

\item Implementation details 

\item Training and OoD datasets 

\item Related works on diffusion models

\item Limitations and scope for future work

\item Detailed quantitative results

\item Additional qualitative results 

\end{enumerate}

\section{Samples from the GenDS dataset}
\label{suppsec: gends}

%The GenDS dataset comprises a total of $7,78,260$ samples, with $2,18,979$ samples for training from existing datasets (excluding validation samples) and $5,59,281$ samples generated using the GenDeg model (Sec.~\ref{subsec: diffmodel}). Fig.~\ref{supfig: gends} shows some generated examples from the GenDS dataset, where the left image is the ground truth and the right image is its degraded version synthesized by GenDeg. For rain, snow and low-light, the ground truth is the clean image reconstructed via the VAE encoding-decoding process, as detailed in Section~\ref{subsec: synthdataset}.

The GenDS dataset comprises a total of $783861$ samples, with $224580$ samples from existing datasets and $559281$ samples generated using the GenDeg model (Sec.~\ref{subsec: diffmodel}). Fig.~\ref{supfig: gends} shows some generated examples from the GenDS dataset, where the left image is the ground truth and the right image is its degraded version synthesized by GenDeg. For rain, snow and low-light, the ground truth is the clean image reconstructed via the VAE encoding-decoding process, as mentioned in Section~\ref{subsec: diffmodel}.

\begin{figure*}
    \centering
    \begin{tabular}{cc}
         \includegraphics[width=0.45\linewidth]{supp_figs/cvpr2025_gends.png}& \includegraphics[width=0.45\linewidth]{supp_figs/cvpr2025_gends_raindrop.png} \\
         
         \includegraphics[width=0.45\linewidth]{supp_figs/cvpr2025_gends_low.png}& \includegraphics[width=0.45\linewidth]{supp_figs/cvpr2025_gends_motion.png} \\

         \includegraphics[width=0.45\linewidth]{supp_figs/cvpr2025_gends_rain.png}& \includegraphics[width=0.45\linewidth]{supp_figs/cvpr2025_gends_snow.png} \\
    \end{tabular}
    \caption{Samples from the GenDS dataset for each degradation type generated using the GenDeg model. The left image is the input clean image, and the right image is its synthesized degraded version.}
    \label{supfig: gends}
\end{figure*}

\section{Conditioning with and without $\mu, \sigma$}
\label{supsec: musigma}

As discussed in Sec.~\ref{sec:proposed}, not conditioning on $\mu$ and $\sigma$ for degradation synthesis results in lack of diversity in the generated degradations. Fig.~\ref{supfig: badsamples} illustrates examples of degradations generated without conditioning on $\mu$ and $\sigma$. These degradations lack the diversity seen in those generated with $\mu$ and $\sigma$ conditioning, as shown in Figure~\ref{supfig: gends}. Specifically, the haze appears excessively thick, the rain is either too intense or too light, and the snow is very faint. 
%We also provide the FID scores for generated images from each degradation for with and without $\mu,\sigma$ conditioning in Table~\ref{suptab: musigma}. FID scores are much better when using $\mu, \sigma$ conditioning.

\begin{figure*}
    \centering
    \includegraphics[width=1\linewidth]{supp_figs/cvpr2025_gends_basamples.png}
    \caption{Samples generated by the diffusion model trained without conditioning on $\mu \text{ and } \sigma$. Samples exhibit limited diversity with degradations having either very high intensity or being very faint.}
    \label{supfig: badsamples}
\end{figure*}

\section{Impact of structure correction $S$}
\label{supsec: scm}

The structure correction module, $S$, discussed in Sec.~\ref{subsec: diffmodel} aims to reverse the structural distortions introduced during the VAE encoding-decoding process. To illustrate its effectiveness, Figure~\ref{supfig: scm} shows examples of generated haze (row 1) and raindrop samples (row 2) before and after applying $S$. The module corrects distortions in the text caused by the VAE encoding-decoding process, thereby improving alignment between the degraded and clean images. The third row in Fig.~\ref{supfig: scm} demonstrates the impact of $S$ on snowy samples. While $S$ successfully preserves structural details, it does not maintain the fine details of the snow, resulting in a blurred appearance of the snow. We observed similar effects for rain and low-light. Hence, we apply $S$ only to haze, motion blur and raindrop samples, as mentioned in Sec.~\ref{subsec: diffmodel}.

\begin{figure*}[t]
\setlength{\tabcolsep}{1pt}
    \centering
    \begin{tabular}{ccc}
         Clean image&Without $S$& With $S$  \\

        \includegraphics[height=3cm, width=5cm]{supp_figs/proc_paper_scm/ds/gtforscm/52_gt.png.png}&  \includegraphics[height=3cm, width=5cm]{supp_figs/proc_paper_scm/ds/noscm/52_noscm.png.png}& \includegraphics[height=3cm, width=5cm]{supp_figs/proc_paper_scm/ds/scm/52_scm.png.png}\\
        
         \includegraphics[height=3cm, width=5cm]{supp_figs/proc_paper_scm/ds/gtforscm/8_gt.jpg.png}&  \includegraphics[height=3cm, width=5cm]{supp_figs/proc_paper_scm/ds/noscm/8_noscm.jpg.png}& \includegraphics[height=3cm, width=5cm]{supp_figs/proc_paper_scm/ds/scm/8_scm.jpg.png}\\

         \includegraphics[height=3cm, width=5cm]{supp_figs/proc_paper_scm/ds/gtforscm/aachen_gt.png.png}&  \includegraphics[height=3cm, width=5cm]{supp_figs/proc_paper_scm/ds/noscm/aachen_noscm.png.png}& \includegraphics[height=3cm, width=5cm]{supp_figs/proc_paper_scm/ds/scm/aachen_scm.png.png}\\
    \end{tabular}
    \caption{Effect of $S$ on haze, raindrop and snow samples. $S$ corrects the structural distortions introduced by the VAE encoding-decoding process.}
    \label{supfig: scm}
\end{figure*}

\section{Dataset filtering thresholds}
\label{supsec: datasetfiltering}

After synthesizing samples using GenDeg, we filter out poor quality samples based on a mean degradation intensity based threshold. Specifically, we calculate the mean intensity, $\mu_\text{filter}$, as the average absolute difference between each generated sample and its corresponding clean image. If $\mu_\text{filter}$ exceeds a certain threshold, $T$, for a given degradation, the sample is discarded.  The threshold values used for each degradation are as follows: $T=0.3$ for haze, $T=0.23$ for rain, $T=0.45$ for snow, $T=0.07$ for motion blur, and $T=0.1$ for raindrop. The thresholds were chosen by visual inspection for each degradation. Using this method, we filtered out approximately $50000$ low-quality samples.

\section{Comparison of $1 \times 1$ and $3\times 3$ convolutions in the Swin decoder}
\label{supsec: swin_decoder}

We observed that employing $3 \times 3$ convolutions in the decoder of the Swin based model significantly mitigates patch border artifacts~\cite{degae}. To validate this, we trained
the Swin model on the GenDS dataset using a decoder with $1\times 1$ convolutions instead of the proposed $3\times 3$ convolutions. Evaluation on the O-Haze~\cite{ohaze} dataset yielded LPIPS/FID scores of $0.186/84.30$, which are substantially worse than the scores obtained with $3\times 3$ convolutions in the decoder ($0.165/74.6$). Fig.~\ref{supfig: 1x1} highlights the presence of patch border artifacts when $1\times 1$ convolutions are used. The artifacts are effectively removed with $3\times 3$ convolutions, as shown in the zoomed-in patches. Furthermore, the decoder with $3\times 3$ convolutions delivers superior dehazing performance, demonstrating its effectiveness.

\begin{figure*}
    \centering
    \setlength{\tabcolsep}{1pt}
    \begin{tabular}{cccc}
         Image&$1\times 1$ convolution&$3\times 3$ convolutions&Ground truth  \\
         \includegraphics[height=0.2\linewidth, width=0.24\linewidth]{supp_figs/proc_supp_1x1/Haze/Real/O-HAZE/input/02_outdoor_GT.png.png}& \includegraphics[height=0.2\linewidth, width=0.24\linewidth]{supp_figs/proc_supp_1x1/Haze/Real/O-HAZE/swin_1x1/02_outdoor_GT.png.png}& \includegraphics[height=0.2\linewidth, width=0.24\linewidth]{supp_figs/proc_supp_1x1/Haze/Real/O-HAZE/Swin GenDS/02_outdoor_GT.png.png}& \includegraphics[height=0.2\linewidth, width=0.24\linewidth]{supp_figs/proc_supp_1x1/Haze/Real/O-HAZE/GT/02_outdoor_GT.png.png} \\
         
         \includegraphics[height=0.2\linewidth, width=0.24\linewidth]{supp_figs/proc_supp_1x1/Haze/Real/O-HAZE/input/8_outdoor_GT.png.png}& \includegraphics[height=0.2\linewidth, width=0.24\linewidth]{supp_figs/proc_supp_1x1/Haze/Real/O-HAZE/swin_1x1/8_outdoor_GT.png.png}& \includegraphics[height=0.2\linewidth, width=0.24\linewidth]{supp_figs/proc_supp_1x1/Haze/Real/O-HAZE/Swin GenDS/8_outdoor_GT.png.png}& \includegraphics[height=0.2\linewidth, width=0.24\linewidth]{supp_figs/proc_supp_1x1/Haze/Real/O-HAZE/GT/8_outdoor_GT.png.png} \\
    \end{tabular}
    \caption{Impact of using $1\times 1$ convolutions in the decoder of the Swin-based model instead of $3\times 3$ convolutions. $3\times 3$ convolutions in the decoder effectively mitigate the patch border artifacts, as shown by the zoomed-in patches.}
    \label{supfig: 1x1}
\end{figure*}

\section{Implementation details}
\label{supsec: impl}

In this section, we provide various implementation details for training GenDeg and the restoration networks.

\textbf{GenDeg. }We use the InstructPix2pix~\cite{ip2p} codebase to train our GenDeg framework, closely following their training strategies. The diffusion model is trained for a total of $60$ epochs with a batch size of $512$, while the structure correction module ($S$) is trained for $8$ epochs with a batch size of $8$, after training the diffusion model. For degradation generation, we use an image guidance scale of $s_I=1.5$ and a text guidance scale of $s_T=7.5$. The guidance scales correspond to those used in InstructPix2pix.

\textbf{Restoration models. }All restoration networks are trained for a total of $50$ epochs using the AdamW optimizer with an initial learning rate of $2 \times 10^{-4}$ and a Cosine annealing learning rate scheduler with linear warmup for $1$ epoch.  PromptIR and NAFNet are trained with batch sizes of $64$ while the Swin model is trained with a batch size of $48$. All models were optimized using $L1$ loss.

\section{Training and OoD datasets}
\label{suppsec: datasets}

We now describe the datasets used to train our degradation generator, GenDeg, and the image restoration models. We also detail the out-of-distribution (OoD) test sets employed for evaluating model generalization. Within-distribution testing is conducted on the test splits of the training datasets unless specified otherwise. For each type of degradation—haze, rain, snow, motion blur, low-light, and raindrops—we utilize both existing datasets and our synthesized data to train the restoration models. Dataset details are given below where R (in brackets ()) indicates real dataset while S indicates synthetic dataset.

\begin{enumerate}
    \item \textbf{Haze}

    \textit{Training Datasets} - DenseHaze~\cite{densehaze} (R) comprising $55$ images of which we use $45$ for training and $10$ for testing, NH-Haze~\cite{nhhaze} (R) comprising $55$ images of which we use $45$ for training and $10$ for testing, I-Haze~\cite{ihaze} (R) comprising 30 images of which we use $25$ for training and $5$ for testing, RESIDE~\cite{reside} (S) comprising $72135$ images for training and $500$ images from the SOTS~\cite{reside} dataset for testing, and FoggyCityscapes~\cite{cityfog} (S) comprising $8925$ images for training and $4575$ images for testing, totaling $81175$ training samples. We further augment these with $113748$ hazy images synthesized by GenDeg .

    \textit{OoD Test Sets} - O-Haze~\cite{ohaze} (R) comprising $45$ images and REVIDE~\cite{revide} (R) comprising $284$ test images.
    
    \item \textbf{Rain}
    
    \textit{Training Datasets} - Real rain split of RainDS~\cite{rainds} (R) comprising $150$ images for training and $98$ images for testing, RealRain1K~\cite{realrain1k} (R) comprising $2100$ images for training and $300$ images for testing, ORD~\cite{ord} (S) comprising $8250$ images for training and $750$ for testing, Rain13K~\cite{mprnet} (S) comprising $13711$ images for training and $4298$ for testing, Rain1400~\cite{rain1400} (S) with $12600$ images for training and $1400$ for testing, and SPAC~\cite{spac} (S) comprising $3124$ images for training and $1690$ images for testing, totaling $39935$ training samples. The images in the ORD dataset are degraded by a mix of haze and rain. These are augmented with an additional $99753$ rainy images synthesized by GenDeg.
    
    \textit{OoD Test Sets} - We evaluate on LHP-Rain~\cite{lhprain} (R) comprising $1000$ test images and the synthetic rain split of RainDS (S) with $200$ test images.
    
    \item \textbf{Snow}
    
    \textit{Training Datasets} - SnowCityscapes~\cite{snowcity} (S) comprising $6000$ images for both training and testing, CSD~\cite{csd} (S) containing $8000$ images for training $2000$ for testing, and Snow100K~\cite{snow100k} (S) with $50000$ images for training and $16801$ images from the Snow100k-L set for testing, totaling $64000$ training samples. The images in the CSD dataset are degraded by a mix of haze and snow. These datasets are augmented with an additional $60516$ snowy images synthesized by GenDeg.
    
    \textit{OoD Test Sets} - RSVD~\cite{rsvd} (S) with $3558$ test samples. The images in the RSVD dataset are degraded by a mix of haze and snow. We could not acquire the RealSnow~\cite{wgws} dataset due to technical difficulties.
    
    \item \textbf{Motion Blur}
    
    \textit{Training Datasets} - HIDE~\cite{hide} (R) with $6397$ images fro training and $2025$ for testing, RealBlur~\cite{realblur} (R) comprising $3758$ images for training and $980$ for testing, and REDS~\cite{reds} (R) with $24000$ training images and $3000$ test images, totaling $34155$ samples for training. We augment these with an additional $79256$ blurry images synthesized by GenDeg.
    
    \textit{OoD Test Sets} - GoPro~\cite{gopro} (R) dataset with $1111$ test images.
    
    \item \textbf{Low-Light}
    
    \textit{Training Datasets} - LOLv2~\cite{lolv2} (R, S) with $1589$ training images and $200$ testing images and SID~\cite{sid} (R) comprising $1865$ images for training and $598$ for testing (Sony images only), totaling $3454$ training samples. These are augmented with an additional $114053$ low-light images synthesized by GenDeg.
    
    \textit{OoD Test Sets} - LOLv1~\cite{lolv1} (R) with $15$ testing samples and SICE~\cite{sice} (R) with $925$ testing samples of which we only use the low-light images (images with index less than $4$).
    
    \item \textbf{Raindrop}
    
    \textit{Training Datasets} - Raindrop dataset~\cite{raindrop} (R) with $861$ training images and $58$ testing images, and the synthetic raindrop split of RainDS~\cite{rainds} (S) with $1000$ training and $200$ testing samples, totaling $1861$ training samples. These are augmented with an additional $91955$ raindrop images synthesized by GenDeg.
    
    \textit{OoD Test Sets} - Real raindrop split of RainDS~\cite{rainds} (R) with $98$ samples for testing.

\end{enumerate}

%Note that the total samples in the existing datasets described above is $2,24,580$ samples. This is different from $2,18,979$ samples mentioned in Sec.~\ref{suppsec: gends} as the validation samples are excluded in Sec.~\ref{suppsec: gends}.

\section{Related works on diffusion models}
\label{supsec: related_diffmodel}
Diffusion models have gained significant attention as generative models, with them being the current state-of-the-art data generators \cite{diffusion1, diffusion2}. In the diffusion process, two processes are learnt. The forward process iteratively adds noise to the data while the denoising (backward) process learns to model the reverse process and gradually denoises the data. Based on this principle, Denoising Diffusion Probabilistic Models (DDPMs) \cite{diffusion2} were proposed that could generate high fidelity images from noise. Various recent advances in diffusion models have extended DDPMs to complex tasks like text-to-image synthesis \cite{stablediff}, conditional synthesis \cite{ip2p} and audio generation \cite{diffusion3}, among others. 

\section{Limitations and scope for future work}
\label{supsec: limitations}

Despite our generated data significantly enhancing the out-of-distribution (OoD) performance of restoration models, we acknowledge some limitations with our data and pipeline. Our approach relies on the Stable Diffusion 1.5~\cite{stablediff} while more recent versions, such as Stable Diffusion 2.0, 3.0 and SDXL~\cite{sdxl}, have since emerged. An interesting research direction would be to explore the domain gap effects and performance improvements offered by these newer versions. Additionally, our structure correction module, $S$, does not perform optimally for snow, rain and low-light (as discussed in Secs.~\ref{supsec: scm} and ~\ref{subsec: diffmodel}). Future research could focus on developing improved correction modules to handle these specific degradations more effectively, to mitigate the structural distortions in the generated degraded images. Furthermore, scaling the synthetic data further and analyzing its impact could be beneficial, as our dataset is still relatively small compared to those used to train foundation models for low-level vision tasks, such as SAM~\cite{sam} and Depth Anything~\cite{depthanything}. Overall, leveraging diffusion models to generate large-scale synthetically degraded images to improve the generalization of image restoration models is a promising research direction.

\section{Detailed quantitative results}
\label{supsec: quant}

In the main paper, we provided out-of-distribution (OoD) performance of methods in terms of LPIPS and FID metrics in Table~\ref{tab: quant_ood}. Subsequently, we provided the mean within-distribution performance of methods for each degradation with LPIPS and FID metrics  (Table.~\ref{tab: quant_within}). This section presents more detailed quantitative evaluations using PSNR, SSIM, LPIPS and FID metrics for within-distribution comparisons, and PSNR and SSIM metrics for OoD comparisons. 

The within-distribution comparisons are provided in detail for each test set described in Sec.~\ref{suppsec: datasets}. Tables~\ref{suptab:quant_withindist_haze},~\ref{suptab:quant_withindist_rain},~\ref{suptab:quant_withindist_snow},~\ref{suptab:quant_withindist_motion},~\ref{suptab:quant_withindist_lowlight},~\ref{suptab:quant_withindist_raindrop} summarize the within-distribution performances for haze, rain, snow, motion blur, low-light and raindrop degradations, respectively. Comparisons with state-of-the-art (SOTA) methods are included if the method is trained for that degradation. From the tables, substantial improvements can be observed for most cases when training with the GenDS dataset for haze, low-light, and raindrop degradations, while competitive performance is maintained for other degradations. Note that some within-distribution datasets might be OoD for SOTA approaches as they were not retrained on all within-distribution datasets. The specific within-distribution datasets for each SOTA approach are given in Table~\ref{suptab:withindist_sota}. 

Table~\ref{suptab: quant_ood_psnrssim} reports PSNR and SSIM metrics for the OoD test sets (LPIPS and FID were provided in Table~\ref{tab: quant_ood} of the main paper). Observe that training with the GenDS datset yields substantial improvements in most cases, particularly in the SSIM scores. However, PSNR is more sensitive to color shifts, which can lower its values despite overall enhancements, as explained in Sec.~\ref{subsec: results}. Furthermore, the SSIM improvement for NAFNet and NAFNet GenDS for the real raindrop split of RainDS dataset is marginal. However, the LPIPS and FID scores in Table~\ref{tab: quant_ood} of the main paper reveal more pronounced improvements. The improvement in LPIPS and FID scores aligns well with the qualitative results for this dataset as shown in Fig.~\ref{fig: qual} of the main paper and Fig.~\ref{supfig: ood_ours}. As LPIPS and FID metrics better correlate with perceptual quality, they are more reliable indicators than PSNR and SSIM~\cite{lpips,stablediff,perceptualbetter1,diffplugin} for assessing OoD performance.

We also provide quantitative results for both within-distribution and OoD test sets
in the form of radar plots in Fig.~\ref{supfig: radars} for ease of viewing.

% Define column types
\newcolumntype{L}{>{\raggedright\arraybackslash}p{2cm}}  % Left-aligned, fixed width for Method
\newcolumntype{C}{>{\centering\arraybackslash}X}       % Centered, flexible width for datasets

\begin{sidewaystable*}[t]
    \centering
    \caption{Quantitative comparisons of various models using PSNR ($\uparrow$), SSIM ($\uparrow$), LPIPS ($\downarrow$) and FID ($\downarrow$) metrics on within-distribution haze datasets. The format of metrics is PSNR/SSIM/LPIPS/FID. PromptIR~\cite{promptir}, NAFNet~\cite{nafnet} and the Swin model are trained with and without the GenDS dataset. The table also includes the performance of existing state-of-the-art (SOTA) all-in-one restoration (AIOR) approaches, namely, DiffUIR~\cite{diffuir}, Diff-Plugin~\cite{diffplugin}, InstructIR~\cite{instructir} and AutoDIR~\cite{autodir}. (R) indicates real image dataset and (S) indicates synthetic image dataset. Diff-Plugin\textsuperscript{\#} is the publicly available pre-trained model.}
    \label{suptab:quant_withindist_haze}
    \setlength{\tabcolsep}{1pt} % Uncomment if you need to reduce column padding
    \small
    \begin{tabularx}{\textwidth}{LCCCCC}
        \toprule
        \textbf{Method} & 
        \textbf{Densehaze~\cite{densehaze}\hspace{0.2cm} (R)} & 
        \textbf{NH-Haze~\cite{nhhaze}\hspace{0.2cm} (R)} & 
        \textbf{I-Haze~\cite{ihaze}\hspace{0.2cm} (R)} & 
        \textbf{RESIDE~\cite{reside}\hspace{0.2cm} (S)} & 
        \textbf{FoggyCityscapes~\cite{cityfog}\hspace{0.2cm} (S)} \\
        \midrule
        DiffUIR & 
        10.20/0.359/0.799/322.58 & 
        12.59/0.498/0.507/220.10 & 
        14.02/0.732/0.208/135.65 & 
        32.94/0.956/0.013/3.71 & 
        18.56/0.834/0.120/25.28 \\
        \hline
        Diff-Plugin\textsuperscript{\#} & 
        10.54/0.363/0.763/326.64 & 
        12.19/0.333/0.523/237.72 & 
        18.36/0.742/0.203/156.08 & 
        23.23/0.765/0.091/21.40 & 
        16.92/0.728/0.178/28.77 \\
        \hline
        InstructIR & 
        10.52/0.436/0.759/336.47 & 
        12.52/0.502/0.511/243.45 & 
        16.05/0.777/0.328/176.45 & 
        26.90/0.952/0.017/5.62 & 
        16.42/0.791/0.161/32.08 \\
        \hline
        AutoDIR & 
        11.69/0.381/0.770/310.78 & 
        13.00/0.519/0.483/218.52 & 
        16.86/0.814/0.168/125.15 & 
        30.98/0.974/0.013/3.81 & 
        19.04/0.846/0.100/23.12 \\
        \hline
        PromptIR & 
        11.11/0.376/0.789/328.71 & 
        12.62/0.494/0.513/221.45 & 
        17.36/0.806/0.191/143.74 & 
        29.13/0.967/0.016/5.28 & 
        28.10/0.961/0.039/6.08 \\
        \hline
        PromptIR GenDS & 
        16.25/0.490/0.561/312.94 & 
        16.07/0.668/0.311/138.88 & 
        20.07/0.857/0.129/99.44 & 
        30.87/0.977/0.014/5.14 & 
        29.08/0.964/0.038/6.34 \\
        \hline
        Swin & 
        16.24/0.458/0.647/332.50 & 
        16.49/0.635/0.386/172.37 & 
        21.87/0.874/0.135/95.23 & 
        36.16/0.987/0.008/2.96 & 
        28.62/0.956/0.044/6.57 \\
        \hline
        Swin GenDS & 
        17.90/0.530/0.516/315.05 & 
        20.31/0.742/0.251/117.14 & 
        22.05/0.883/0.110/87.39 & 
        38.08/0.989/0.007/2.81 & 
        33.45/0.972/0.027/3.82 \\
        \hline
        NAFNet & 
        16.99/0.517/0.518/327.77 & 
        18.11/0.714/0.276/152.80 & 
        21.33/0.867/0.127/104.00 & 
        32.31/0.981/0.011/3.26 & 
        33.40/0.979/0.021/3.30 \\
        \hline
        NAFNet GenDS & 
        17.67/0.545/0.474/316.06 & 
        19.10/0.743/0.242/109.51 & 
        20.57/0.869/0.109/89.96 & 
        34.80/0.986/0.008/2.88 & 
        32.55/0.977/0.024/3.76 \\
        \hline
        DA-CLIP&10.57/0.348/0.8299/327.52&12.74/0.455/0.544/224.42&16.99/0.737/0.2160/146.69&24.91/0.943/0.025/5.80&19.01/0.863/0.1090/31.32\\
        \hline
        DA-CLIP GenDS&13.25/0.404/0.7019/232.87&15.17/0.568/0.3914/160.4&18.97/0.777/0.1878/135.08&29.73/0.972/0.012/4.00&25.00/0.942/0.045/13.21\\
        \hline
        Diff-Plugin &9.13/0.341/0.796/341.31&13.10/0.331/0.4586/206.70&16.83/0.707/0.2239/129.80&21.56/0.750/0.0997/21.86&19.57/0.776/0.1225/18.67\\
        \hline
        Diff-Plugin GenDS &9.33/0.359/0.7199/331.67&14.24/0.357/0.3942/156.41&16.74/0.718/0.1972/121.15&23.35/0.771/0.0908/20.91&22.12/0.798/0.1094/9.94\\
        
        \bottomrule
    \end{tabularx}
\end{sidewaystable*}

\begin{sidewaystable*}[t]
    \centering
    \caption{Quantitative comparisons of various models using PSNR ($\uparrow$), SSIM ($\uparrow$), LPIPS ($\downarrow$) and FID ($\downarrow$) metrics on within-distribution rain datasets. The format of metrics is PSNR/SSIM/LPIPS/FID. PromptIR~\cite{promptir}, NAFNet~\cite{nafnet} and the Swin model are trained with and without the GenDS dataset. The table also includes the performance of existing state-of-the-art (SOTA) AIOR approaches, namely, DiffUIR~\cite{diffuir}, Diff-Plugin~\cite{diffplugin}, InstructIR~\cite{instructir} and AutoDIR~\cite{autodir}. (R) indicates real image dataset and (S) indicates synthetic image dataset. Diff-Plugin\textsuperscript{\#} is the publicly available pre-trained model.}
    \small
    \label{suptab:quant_withindist_rain}
    \begin{tabularx}{\textwidth}{LCCCCCC}  % 'L' for Method, 'C' for datasets
        \toprule
        \textbf{Method} & 
        \textbf{RainDS~\cite{rainds}\hspace{0.2cm} (R)} & 
        \textbf{Realrain1k~\cite{realrain1k}\hspace{0.2cm} (R)} & 
        \textbf{ORD~\cite{ord}\hspace{0.2cm} (S)} & 
        \textbf{Rain13K~\cite{mprnet}\hspace{0.2cm} (S)} & 
        \textbf{Rain1400~\cite{rain1400}\hspace{0.2cm} (S)} & 
        \textbf{SPAC~\cite{spac}\hspace{0.2cm} (S)} \\
        \midrule
        DiffUIR & 
        25.70/0.802/0.145/49.36 & 
        27.02/0.905/0.088/18.23 & 
        16.82/0.644/0.385/143.1 & 
        31.03/0.904/0.069/14.10 & 
        27.76/0.899/0.141/42.54 & 
        23.70/0.803/0.223/53.81 \\
        \hline
        Diff-Plugin\textsuperscript{\#} & 
        21.39/0.526/0.215/60.65 & 
        24.14/0.660/0.150/35.00 & 
        13.39/0.470/0.423/94.62 & 
        21.71/0.617/0.169/26.86 & 
        22.27/0.623/0.155/46.61 & 
        24.46/0.733/0.118/18.86 \\
        \hline
        InstructIR & 
        25.41/0.789/0.151/51.93 & 
        30.71/0.939/0.067/16.70 & 
        13.37/0.565/0.436/89.21 & 
        29.56/0.885/0.088/16.06 & 
        30.97/0.907/0.071/25.09 & 
        31.97/0.951/0.055/11.23 \\
        \hline
        AutoDIR & 
        24.87/0.773/0.161/69.21 & 
        30.04/0.924/0.079/18.21 & 
        14.29/0.594/0.394/93.56 & 
        30.52/0.895/0.073/12.65 & 
        31.18/0.913/0.055/17.64 & 
        31.69/0.941/0.077/17.49 \\
        \hline
        PromptIR & 
        24.28/0.759/0.157/75.87 & 
        32.85/0.922/0.095/19.47 & 
        25.53/0.863/0.124/47.54 & 
        29.85/0.884/0.089/17.45 & 
        30.69/0.901/0.073/26.23 & 
        33.07/0.958/0.045/9.14 \\
        \hline
        PromptIR GenDS & 
        25.36/0.788/0.135/50.35 & 
        32.02/0.917/0.103/19.54 & 
        26.45/0.866/0.135/48.05 & 
        30.17/0.888/0.010/18.41 & 
        31.11/0.908/0.072/24.82 & 
        34.32/0.964/0.030/6.54 \\
        \hline
        Swin & 
        25.63/0.793/0.151/47.10 & 
        33.26/0.936/0.065/14.47 & 
        27.39/0.859/0.150/39.30 & 
        30.89/0.898/0.085/15.84 & 
        31.16/0.909/0.070/23.71 & 
        33.82/0.959/0.031/6.62 \\
        \hline
        Swin GenDS & 
        25.97/0.794/0.149/46.46 & 
        34.15/0.951/0.054/13.25 & 
        28.31/0.867/0.134/36.88 & 
        30.62/0.894/0.098/17.96 & 
        30.98/0.907/0.071/25.07 & 
        33.37/0.957/0.037/7.29 \\
        \hline
        NAFNet & 
        25.73/0.798/0.134/45.92 & 
        34.98/0.951/0.055/14.71 & 
        29.18/0.896/0.089/29.65 & 
        31.22/0.904/0.078/14.48 & 
        31.73/0.917/0.063/21.36 & 
        34.59/0.966/0.026/4.94 \\
        \hline
        NAFNet GenDS & 
        25.94/0.800/0.130/41.22 & 
        34.28/0.947/0.059/14.46 & 
        29.02/0.893/0.104/33.43 & 
        31.23/0.906/0.0792/15.22 & 
        31.56/0.916/0.0661/22.80 & 
        34.78/0.967/0.029/5.66 \\
        DA-CLIP&22.46/0.660/0.1672/55.98&24.71/0.871/0.1087/21.90&20.80/0.778/0.1494/43.72&25.71/0.822/0.1062/32.00&26.28/0.841/0.0884/28.10&28.24/0.926/0.065/18.23\\
         \hline
         DA-CLIP GenDS&23.32/0.652/0.1941/61.30&28.28/0.883/0.1017/20.28&23.75/0.821/0.1124/38.60&28.38/0.852/0.0887/26.74&28.92/0.866/0.0764/25.24&32.57/0.944/0.0389/10.89\\
         \hline
         Diff-Plugin&21.14/0.522/0.2078/58.28&23.88/0.667/0.1421/33.94&18.05/0.570/0.2070/56.78&21.75/0.620/0.1645/26.32&22.23/0.624/0.1542/44.51&24.39/0.739/0.1127/18.47\\
        \hline
         Diff-Plugin GenDS&21.70/0.530/0.1989/54.25&24.33/0.676/0.1395/32.81&17.18/0.555/0.2268/58.42&21.89/0.621/0.1647/26.54&22.40/0.626/0.1544/45.32&24.72/0.741/0.1047/18.01\\
        \bottomrule
    \end{tabularx}
\end{sidewaystable*}

\begin{table*}[t]
    \centering
    \caption{Quantitative comparisons of various models using PSNR ($\uparrow$), SSIM ($\uparrow$), LPIPS ($\downarrow$) and FID ($\downarrow$) metrics on within-distribution snow datasets. The format of metrics is PSNR/SSIM/LPIPS/FID. PromptIR~\cite{promptir}, NAFNet~\cite{nafnet} and the Swin model are trained with and without the GenDS dataset. The table also includes the performance of existing state-of-the-art (SOTA) AIOR approaches, namely, DiffUIR~\cite{diffuir} and Diff-Plugin~\cite{diffplugin}. (R) indicates real image dataset and (S) indicates synthetic image dataset. Diff-Plugin\textsuperscript{\#} is the publicly available pre-trained model.}
    \small
    \label{suptab:quant_withindist_snow}
    \setlength{\tabcolsep}{1pt} % Uncomment if you need to reduce column padding
    \begin{tabularx}{0.8\textwidth}{L C C C}  % 'L' for Method, 'C' for datasets
        \toprule
        \textbf{Method} & 
        \textbf{SnowCityscapes~\cite{snowcity}\hspace{0.2cm} (S)} & 
        \textbf{CSD~\cite{csd}\hspace{0.2cm} (S)} & 
        \textbf{Snow100k~\cite{snow100k}\hspace{0.2cm} (S)} \\
        \midrule
        DiffUIR & 
        12.42/0.330/0.583/20.16 & 
        17.57/0.790/0.196/43.81 & 
        28.76/0.869/0.138/7.05 \\
        \hline
        Diff-Plugin\textsuperscript{\#} & 
        22.25/0.694/0.242/35.35 & 
        15.61/0.635/0.243/41.14 & 
        21.02/0.611/0.196/4.10 \\
        \hline
        PromptIR & 
        30.16/0.918/0.109/26.31 & 
        27.62/0.919/0.071/23.34 & 
        27.86/0.863/0.120/5.39 \\
        \hline
        PromptIR GenDS & 
        31.44/0.934/0.089/19.73 & 
        28.03/0.920/0.070/23.92 & 
        28.51/0.874/0.115/4.92 \\
        \hline
        NAFNet & 
        33.67/0.953/0.063/7.23 & 
        31.92/0.947/0.044/14.13 & 
        30.01/0.893/0.096/3.25 \\
        \hline
        NAFNet GenDS & 
        33.02/0.950/0.061/6.96 & 
        31.39/0.942/0.048/15.36 & 
        29.78/0.891/0.100/3.38 \\
        \hline
        Swin & 
        32.38/0.934/0.081/9.41 & 
        32.01/0.935/0.058/19.13 & 
        29.34/0.880/0.104/3.87 \\
        \hline
        Swin GenDS & 
        32.17/0.929/0.085/9.46 & 
        31.95/0.933/0.059/20.52 & 
        29.23/0.881/0.107/4.34 \\
        \hline
        DA-CLIP&25.42/0.849/0.1574/53.67&22.72/0.872/0.092/32.25&24.31/0.803/0.1350/44.92\\
        \hline
        DA-CLIP GenDS&31.51/0.937/0.057/22.88&27.15/0.916/0.057/21.92&27.16/0.853/0.1037/34.65\\
        \hline
        Diff-Plugin&23.05/0.718/0.1932/15.63&20.21/0.699/0.1559/30.66&21.38/0.617/0.1855/7.95\\
        \hline
        Diff-Plugin GenDS&22.19/0.716/0.1823/13.45&19.08/0.691/0.1606/31.69&20.43/0.613/0.1866/7.96\\

        \bottomrule
    \end{tabularx}
\end{table*}

\begin{table*}[t]
    \centering
    \caption{Quantitative comparisons of various models using PSNR ($\uparrow$), SSIM ($\uparrow$), LPIPS ($\downarrow$) and FID ($\downarrow$) metrics on within-distribution motion blur datasets. The format of metrics is PSNR/SSIM/LPIPS/FID. PromptIR~\cite{promptir}, NAFNet~\cite{nafnet} and the Swin model are trained with and without the GenDS dataset. The table also includes the performance of existing state-of-the-art (SOTA) AIOR approaches, namely, DiffUIR~\cite{diffuir}, Diff-Plugin~\cite{diffplugin}, InstructIR~\cite{instructir} and AutoDIR~\cite{autodir}. (R) indicates real image dataset and (S) indicates synthetic image dataset. Diff-Plugin\textsuperscript{\#} is the publicly available pre-trained model.}
    \small
    \label{suptab:quant_withindist_motion}
    \setlength{\tabcolsep}{1pt} % Uncomment if you need to reduce column padding
    \begin{tabularx}{0.8\textwidth}{L C C C}  % 'L' for Method, 'C' for datasets
        \toprule
        \textbf{Method} & 
        \textbf{HIDE~\cite{hide}\hspace{0.2cm} (R)} & 
        \textbf{RealBlur~\cite{realblur}\hspace{0.2cm} (R)} & 
        \textbf{REDS~\cite{reds}\hspace{0.2cm} (R)} \\
        \midrule
        DiffUIR & 
        27.17/0.854/0.174/26.23 & 
        26.15/0.721/0.188/44.80 & 
        26.84/0.825/0.185/57.64 \\
        \hline
        Diff-Plugin\textsuperscript{\#} & 
        21.40/0.658/0.247/39.68 & 
        23.62/0.728/0.192/43.65 & 
        21.47/0.628/0.216/68.40 \\
        \hline
        InstructIR & 
        27.50/0.859/0.165/21.37 & 
        27.09/0.845/0.127/25.39 & 
        26.93/0.831/0.154/48.82 \\
        \hline
        AutoDIR & 
        27.03/0.862/0.170/21.67 & 
        24.77/0.770/0.149/28.58 & 
        27.23/0.846/0.167/49.77 \\
        \hline
        PromptIR & 
        26.55/0.837/0.190/30.07 & 
        28.13/0.845/0.168/35.78 & 
        29.45/0.867/0.133/41.52 \\
        \hline
        PromptIR GenDS & 
        26.70/0.845/0.204/30.29 & 
        28.44/0.857/0.165/32.81 & 
        29.58/0.871/0.146/41.70 \\
        \hline
        NAFNet & 
        27.40/0.864/0.164/25.66 & 
        28.93/0.876/0.140/27.41 & 
        30.94/0.898/0.105/33.10 \\
        \hline
        NAFNet GenDS & 
        27.53/0.866/0.163/26.68 & 
        29.03/0.879/0.138/27.68 & 
        30.82/0.896/0.110/33.59 \\
        \hline
        Swin & 
        25.91/0.829/0.226/34.35 & 
        28.15/0.851/0.182/39.60 & 
        29.23/0.866/0.176/48.14 \\
        \hline
        Swin GenDS & 
        25.89/0.830/0.196/34.24 & 
        28.44/0.854/0.228/48.39 & 
        29.01/0.866/0.145/43.88 \\
        \hline
        DA-CLIP&22.03/0.743/0.2139/49.65&24.50/0.719/0.1928/45.40&24.37/0.779/0.1884/55.06\\
         \hline
        DA-CLIP GenDS&23.95/0.778/0.1620/39.37&27.52/0.825/0.1236/31.36&27.04/0.805/0.1342/42.74\\
         \hline
        Diff-Plugin&22.18/0.694/0.1673/27.61&25.40/0.764/0.1302/28.89&22.80/0.647/0.1445/56.56\\
        \hline
        Diff-Plugin GenDS&22.68/0.706/0.1599/25.74&25.81/0.772/0.1248/26.61&22.78/0.649/0.1414/55.62\\
        \bottomrule
    \end{tabularx}
\end{table*}

\begin{table*}[t]
    \centering
    \caption{Quantitative comparisons of various models using PSNR ($\uparrow$), SSIM ($\uparrow$), LPIPS ($\downarrow$) and FID ($\downarrow$) metrics on within-distribution low-light datasets. The format of metrics is PSNR/SSIM/LPIPS/FID. PromptIR~\cite{promptir}, NAFNet~\cite{nafnet} and the Swin model are trained with and without the GenDS dataset. The table also includes the performance of existing state-of-the-art (SOTA) AIOR approaches, namely, DiffUIR~\cite{diffuir}, Diff-Plugin~\cite{diffplugin}, InstructIR~\cite{instructir} and AutoDIR~\cite{autodir}. (R) indicates real image dataset and (S) indicates synthetic image dataset. Diff-Plugin\textsuperscript{\#} is the publicly available pre-trained model.}
    \small
    \label{suptab:quant_withindist_lowlight}
    \setlength{\tabcolsep}{1pt} % Uncomment if you need to reduce column padding
    \begin{tabularx}{0.6\textwidth}{L C C}  % 'L' for Method, 'C' for datasets
        \toprule
        \textbf{Method} & 
        \textbf{LOLv2~\cite{lolv2}\hspace{0.2cm} (R, S)} & 
        \textbf{{SID~\cite{sid}\hspace{0.2cm}} (R
        )} \\
        \midrule
        DiffUIR & 
        20.27/0.826/0.204/64.17 & 
        9.86/0.061/0.899/456.35 \\
        \hline
        Diff-Plugin\textsuperscript{\#} & 
        18.00/0.644/0.226/62.83 & 
        12.47/0.365/0.703/298.52 \\
        \hline
        InstructIR & 
        23.99/0.857/0.156/46.28 & 
        12.84/0.377/0.649/269.21 \\
        \hline
        AutoDIR & 
        19.94/0.800/0.176/48.02 & 
        13.45/0.457/0.665/262.27 \\
        \hline
        PromptIR & 
        17.25/0.710/0.264/76.65 & 
        17.67/0.517/0.579/303.10 \\
        \hline
        PromptIR GenDS & 
        21.90/0.868/0.142/51.75 & 
        18.31/0.550/0.566/285.43 \\
        \hline
        NAFNet & 
        22.54/0.866/0.140/49.89 & 
        18.13/0.557/0.558/294.83 \\
        \hline
        NAFNet GenDS & 
        22.87/0.887/0.120/38.55 & 
        18.64/0.586/0.514/258.75 \\
        \hline
        Swin & 
        21.97/0.844/0.195/70.92 & 
        17.12/0.517/0.647/304.38 \\
        \hline
        Swin GenDS & 
        22.32/0.869/0.146/49.53 & 
        16.18/0.483/0.591/282.73 \\
        \hline
        DA-CLIP&12.29/0.601/0.2635/76.16&11.21/0.131/0.814/340.79\\
        \hline
        DA-CLIP GenDS&16.31/0.692/0.235/63.16&10.84/0.146/0.633/301.16\\
        \hline  
        Diff-Plugin&16.80/0.594/0.2906/85.27&13.02/0.288/0.6424/250.00\\
        \hline
        Diff-Plugin GenDS&17.96/0.630/0.246/77.87&12.69/0.291/0.666/234.50\\
        \bottomrule
    \end{tabularx}
\end{table*}

\begin{table*}[t]
    \centering
    \caption{Quantitative comparisons of various models using PSNR ($\uparrow$), SSIM ($\uparrow$), LPIPS ($\downarrow$) and FID ($\downarrow$) metrics on within-distribution raindrop datasets. The format of metrics is PSNR/SSIM/LPIPS/FID. PromptIR~\cite{promptir}, NAFNet~\cite{nafnet} and the Swin model are trained with and without the GenDS dataset. The table also includes the performance of an existing state-of-the-art (SOTA) AIOR approach, namely, AutoDIR~\cite{autodir}. (R) indicates real image dataset and (S) indicates synthetic image dataset.}
    \small
    \label{suptab:quant_withindist_raindrop}
    \setlength{\tabcolsep}{1pt} % Uncomment if you need to reduce column padding
    \begin{tabularx}{0.6\textwidth}{L C C}  % 'L' for Method, 'C' for datasets
        \toprule
        \textbf{Method} & 
        \textbf{Raindrop~\cite{raindrop}\hspace{0.2cm} (R)} & 
        \textbf{RainDS~\cite{rainds}\hspace{0.2cm} (S)}\\
        \midrule
        AutoDIR & 
        30.10/0.924/0.058/25.53 & 
        20.22/0.795/0.333/110.66 \\
        \hline
        PromptIR & 
        27.04/0.885/0.120/80.07 & 
        21.76/0.852/0.259/88.90 \\
        \hline
        PromptIR GenDS & 
        29.15/0.908/0.071/45.40 & 
        20.91/0.829/0.305/103.91 \\
        \hline
        NAFNet & 
        29.61/0.914/0.083/48.30 & 
        28.23/0.924/0.088/31.52 \\
        \hline
        NAFNet GenDS & 
        30.33/0.922/0.056/30.42 & 
        28.26/0.927/0.084/29.43 \\
        \hline
        Swin & 
        28.74/0.903/0.089/53.30 & 
        26.98/0.893/0.105/40.88 \\
        \hline
        Swin GenDS & 
        28.89/0.901/0.081/42.54 & 
        26.87/0.893/0.104/36.72 \\
        \hline
        DA-CLIP&25.35/0.861/0.086/43.79&23.98/0.888/0.1175/37.86\\
        \hline
        DA-CLIP GenDS&28.44/0.891/0.0658/32.36&25.23/0.907/0.1212/39.70\\
        \hline
        Diff-Plugin&21.95/0.675/0.1716/71.91&21.21/0.635/0.1990/49.38\\
        \hline
        Diff-Plugin GenDS&25.03/0.733/0.1117/46.76&22.48/0.683/0.1550/38.29\\
        \bottomrule
    \end{tabularx}
\end{table*}

\newcolumntype{C}{>{\centering\arraybackslash}X}

\begin{table*}[t]
    \centering
    \caption{Quantitative comparisons of NAFNet~\cite{nafnet}, PromptIR~\cite{promptir}, and Swin-transformer models using PSNR and SSIM metrics (higher is better), trained with and without our GenDS dataset. Performance is evaluated on OoD test sets. The table also includes the performance of existing state-of-the-art (SOTA) AIOR approaches, namely, DiffUIR~\cite{diffuir}, Diff-Plugin~\cite{diffplugin}, InstructIR~\cite{instructir} and AutoDIR~\cite{autodir}. (R) indicates real images and (S) indicates synthetic images. '-' indicates that the method was not trained for that degradation. Diff-Plugin\textsuperscript{\#} is the publicly available pre-trained model.}
    \small
    \label{suptab: quant_ood_psnrssim}
    \begin{tabularx}{\textwidth}{l *{9}{C}}  % 'l' for Method, 'C' for others
        \toprule
        \textbf{Method} & 
        \textbf{REVIDE \cite{revide}} & 
        \textbf{O-Haze \cite{ohaze} } & 
        \textbf{RainDS \cite{rainds} } & 
        \textbf{LHP \cite{lhprain} } & 
        \textbf{RSVD \cite{rsvd} } & 
        \textbf{GoPro \cite{gopro} } & 
        \textbf{LOLv1 \cite{lolv1} } & 
        \textbf{SICE \cite{sice} } & 
        \textbf{RainDS \cite{rainds} } \\
        \midrule

        \textbf{Degradation Type} & 
        Haze (R) & 
        Haze (R) & 
        Rain (S)& 
        Rain (R)& 
        Snow (S)& 
        Motion Blur (R)& 
        Low-light (R)& 
        Low-light (R)& 
        Raindrop (R)\\
        \midrule
        
        DiffUIR & 
        17.26/0.792 & 
         16.59/0.705& 
         30.85/0.897& 
         26.71/0.832& 
         21.60/0.823& 
         29.17/0.864& 
         21.65/0.836& 
        10.00/0.367 & 
        - \\
        
        Diff-Plugin\textsuperscript{\#} & 
         17.45/0.728& 
         15.79/0.471& 
         22.04/0.635& 
         26.02/0.735& 
        18.92/0.662& 
         21.76/0.633& 
         19.38/0.713& 
         17.59/0.611& 
        - \\
        
        InstructIR & 
         16.51/0.831& 
         16.56/0.709& 
         30.24/0.879& 
         28.93/0.871& 
        - & 
         28.26/0.870& 
         22.81/0.836& 
         17.58/0.750& 
        - \\
        
        AutoDIR & 
         16.31/0.782& 
         17.57/0.731& 
         29.14/0.858& 
         28.44/0.841& 
        - & 
        27.07/0.828 & 
         20.53/0.850& 
         15.37/0.685& 
         23.33/0.754\\
        \midrule
        
        PromptIR & 
         17.56/0.786& 
         16.46/0.701& 
         29.70/0.871& 
         25.85/0.835& 
         20.08/0.838& 
        26.98/0.828& 
         20.53/0.768& 
         12.42/0.438& 
         20.94/0.709\\
        
        PromptIR GenDS & 
         19.20/0.827& 
         22.40/0.849& 
         30.00/0.884& 
         26.15/0.840& 
         21.77/0.858& 
         27.28/0.843& 
         21.38/0.812& 
         11.41/0.466& 
         22.04/0.718\\
        
        Swin & 
         18.44/0.812& 
         20.12/0.802& 
         28.50/0.863& 
         28.97/0.863& 
        22.05/0.838& 
         26.79/0.843& 
         20.07/0.784& 
        15.27/0.667& 
         22.34/0.726\\
        
        Swin GenDS & 
         18.69/0.831& 
         20.60/0.843& 
         29.34/0.868& 
        29.30/0.869& 
         23.07/0.863& 
         26.09/0.830& 
         24.27/0.842& 
         16.05/0.678& 
         22.87/0.740\\
        
        NAFNet & 
         18.71/0.819& 
         19.85/0.814& 
        28.49/0.887& 
         27.41/0.835& 
         21.32/0.848& 
         28.14/0.868& 
         22.37/0.826& 
        14.03/0.592& 
         22.91/0.745\\
        
        NAFNet GenDS & 
         20.96/0.871& 
         20.51/0.849& 
         30.40/0.891& 
         27.53/0.848& 
         22.81/0.873& 
         27.80/0.864& 
         22.82/0.838& 
        14.65/0.614& 
         23.31/0.747\\

         DA-CLIP 
         &16.98/0.758&16.04/0.609& 
        24.74/0.764&25.64/0.838& 
         20.72/0.788& 
         22.87/0.763& 
         10.94/0.474&12.04/0.499& 
         20.99/0.622\\
        
        DA-CLIP GenDS & 
         17.78/0.810&19.94/0.700& 
         25.50/0.758&28.74/0.851& 
         21.42/0.802& 
         25.55/0.795& 
         11.21/0.481& 
        12.02/0.506& 
         21.39/0.621\\

         Diff-Plugin & 
         17.84/0.748&16.36/0.464&
       22.00/0.637&25.10/0.723& 
         19.12/0.663& 
         22.23/0.654& 
         17.77/0.651&18.60/0.588& 
         18.47/0.453\\
        
        Diff-plugin GenDS & 
         17.14/0.765&16.54/0.460& 
         21.89/0.636&26.05/0.739& 
         19.39/0.674& 
         22.84/0.674& 
         18.29/0.676&19.47/0.623& 
         19.54/0.489\\
        \bottomrule
    \end{tabularx}
\end{table*}

% Define column types
\newcolumntype{L}{>{\raggedright\arraybackslash}p{3cm}}  % Left-aligned, fixed width for Method
\newcolumntype{C}{>{\centering\arraybackslash}X}       % Centered, flexible width for datasets

\begin{table*}[t]
    \centering
    \caption{Within-distribution datasets of SOTA AIOR approaches.}
    \small
    \label{suptab:withindist_sota}
    \setlength{\tabcolsep}{1pt} % Reduce column padding if necessary
    \begin{tabularx}{\textwidth}{L C}  % 'L' for Method, 'C' for datasets
        \toprule
        \textbf{Method} & \textbf{Within-distribution Datasets} \\
        \midrule
        DiffUIR~\cite{diffuir} & RESIDE~\cite{reside} (Haze), Rain13K~\cite{mprnet} and Rain1400~\cite{rain1400} (Rain), Snow100k~\cite{snow100k} (Snow), GoPro~\cite{gopro} (Motion blur), LOLv1~\cite{lolv1} (low-light) \\
        
        Diff-Plugin~\cite{diffplugin} & RESIDE~\cite{reside} (Haze), Rain13K~\cite{mprnet} and Rain1400~\cite{rain1400} (Rain), Snow100k~\cite{snow100k} (Snow), GoPro~\cite{gopro} (Motion blur), LOLv1~\cite{lolv1} (low-light) \\
        
        InstructIR~\cite{instructir} & RESIDE~\cite{reside} (Haze), Rain13K~\cite{mprnet} and Rain1400~\cite{rain1400} (Rain), GoPro~\cite{gopro} (Motion blur), LOLv1~\cite{lolv1} (low-light) \\
        
        AutoDIR~\cite{autodir} & RESIDE~\cite{reside} (Haze), Rain13K~\cite{mprnet} and Rain1400~\cite{rain1400} (Rain), GoPro~\cite{gopro} (Motion blur), LOLv1~\cite{lolv1} (low-light) and Raindrop~\cite{raindrop} (Raindrop) \\
        \bottomrule
    \end{tabularx}
\end{table*}

\begin{figure*}
    \centering
    \setlength{\tabcolsep}{1pt}
    \begin{tabular}{cccc}
         \includegraphics[height=4cm, width=4.5cm]{figs/radars_new/Haze_LPIPS.png}&\includegraphics[height=4cm, width=4.5cm]{figs/radars_new/Haze_FID.png}&\includegraphics[height=4cm, width=4cm]{figs/radars_new/Rain_LPIPS.png}&\includegraphics[height=4cm, width=4cm]{figs/radars_new/Rain_FID.png}\\

         \includegraphics[height=4cm, width=4.5cm]{figs/radars_new/Snow_LPIPS.png}&\includegraphics[height=4cm, width=4.5cm]{figs/radars_new/Snow_FID.png}&\includegraphics[height=4cm, width=4cm]{figs/radars_new/Motion Blur_LPIPS.png}&\includegraphics[height=4cm, width=4cm]{figs/radars_new/Motion Blur_FID.png}\\
         
         \includegraphics[height=4cm, width=4cm]{figs/radars_new/Raindrop_LPIPS.png}&\includegraphics[height=4cm, width=4cm]{figs/radars_new/Raindrop_FID.png}& \includegraphics[height=4cm, width=4cm]{figs/radars_new/Low-light_LPIPS.png}&\includegraphics[height=4cm, width=4cm]{figs/radars_new/Low-light_FID.png}\\
         
    \end{tabular}
    \caption{Comparison of NAFNet~\cite{nafnet}, PromptIR~\cite{promptir}, and Swin-transformer models using LPIPS and FID metrics, trained with and without our GenDS dataset. Performance is evaluated on within-distribution (\textcolor{green}{green}) and OoD (\textcolor{red}{red}) test sets. The figure also includes the performance of existing state-of-the-art (SOTA) all-in-one restoration (AIOR) approaches, namely, DiffUIR~\cite{diffuir}, Diff-Plugin~\cite{diffplugin}, InstructIR~\cite{instructir}, and AutoDIR~\cite{autodir}. Training with the GenDS dataset significantly enhances OoD performance. Legend is located in the lower-right corner. Metric values decrease outward.}
    \label{supfig: radars}
    \vskip-8pt
\end{figure*}

\section{Additional qualitative results}
\label{supsec: addnqual}

%showcasing hte improvement obtained when using the GenDS dataset for OoD performance. Additionally, we also show qualitative results for within-distribution performance. Finally, we show qualitative comparisons on OoD performance with SOTA approaches. 
In this section, we provide additional qualitative results. Fig.~\ref{supfig: ood_ours} presents qualitative comparisons of three top-performing image restoration models- PromptIR~\cite{promptir}, Swin model (Sec.~\ref{subsec: genirmodel}) and NAFNet~\cite{nafnet}, evaluated on OoD test sets when trained with and without the GenDS dataset. It can be observed that training with the GenDS dataset results in improved performance. Figure~\ref{supfig: within_dist_ours} illustrates the within-distribution performance of the same models, showing that training with the GenDS dataset yields significant improvements for haze, low-light, and raindrop degradations, while performance remains nearly identical for other degradation types.  This indicates that the GenDS dataset does not degrade within-distribution performance.

Finally, Figs.~\ref{supfig:ood_others},~\ref{supfig:ood_others_snow} and~\ref{supfig:ood_others_raindrop} provide qualitative comparisons of top-performing approaches PromptIR, the Swin model, and NAFNet trained with the GenDS dataset against several SOTA approaches, namely, DiffUIR~\cite{diffuir}, Diff-Plugin~\cite{diffplugin}, InstructIR~\cite{instructir}, and AutoDIR~\cite{autodir}. Diff-Plugin used for qualitative comparisons is the publicly available pre-trained model. Fig.~\ref{supfig:ood_others} shows comparisons for haze, low-light, rain and motion blur, Fig.~\ref{supfig:ood_others_snow} for snow and Fig.~\ref{supfig:ood_others_raindrop} for raindrop removal. These comparisons are split across multiple figures because not all SOTA methods are trained for every degradation task. The models trained on GenDS dataset deliver consistently good OoD performance across all degradations whereas each SOTA approach tends to perform well only for specific degradation types. It is important to note that the primary aim of our approach is not to compete directly with SOTA models, but rather demonstrate the performance differences observed for OoD testing when models are trained with and without the proposed GenDS dataset. Furthermore, training SOTA models on our GenDS dataset may also boost their OoD performance.

\begin{figure*}
    \centering
    \small
    \setlength{\tabcolsep}{1pt}
    \begin{tabular}{ccccccc}
         &Haze&Raindrop&Low-light&Motion blur&Rain&Snow \\

         \rotatebox[origin=c]{90}{Input\hspace{-56pt}}&\includegraphics[height=2.25cm, width=2.75cm]{supp_figs/proc_supp_ood_ours/Haze/Real/REVIDE/input/00057.JPG.png} &\includegraphics[height=2.25cm, width=2.75cm]{supp_figs/Raindrop_topbox/Real/RainDS/input/14.png.png} &\includegraphics[height=2.25cm, width=2.75cm]{supp_figs/proc_supp_ood_ours/Low-light/Real/LOLv1/input/55.JPG.png}&\includegraphics[height=2.25cm, width=2.75cm]{supp_figs/proc_supp_ood_ours/Motion_blur/Real/GoPro/input/003045.png.png}&\includegraphics[height=2.25cm, width=2.75cm]{supp_figs/proc_supp_ood_ours/Rain/Real/LHP/input/10_0.png.png}&\includegraphics[height=2.25cm, width=2.75cm]{supp_figs/proc_supp_ood_ours/Snow/Synthetic/RSVD/input/0127.png.png}\\

         \rotatebox[origin=c]{90}{PromptIR\hspace{-56pt}}& \includegraphics[height=2.25cm, width=2.75cm]{supp_figs/proc_supp_ood_ours/Haze/Real/REVIDE/PromptIR/00057.JPG.png} &\includegraphics[height=2.25cm, width=2.75cm]{supp_figs/Raindrop_topbox/Real/RainDS/PromptIR/14.png.png}&\includegraphics[height=2.25cm, width=2.75cm]{supp_figs/proc_supp_ood_ours/Low-light/Real/LOLv1/PromptIR/55.JPG.png}&\includegraphics[height=2.25cm, width=2.75cm]{supp_figs/proc_supp_ood_ours/Motion_blur/Real/GoPro/PromptIR/003045.png.png}&\includegraphics[height=2.25cm, width=2.75cm]{supp_figs/proc_supp_ood_ours/Rain/Real/LHP/PromptIR/10_0.png.png}&\includegraphics[height=2.25cm, width=2.75cm]{supp_figs/proc_supp_ood_ours/Snow/Synthetic/RSVD/PromptIR/0127.png.png}\\

         \rotatebox[origin=c]{90}{PromptIR GD\hspace{-56pt}}& \includegraphics[height=2.25cm, width=2.75cm]{supp_figs/proc_supp_ood_ours/Haze/Real/REVIDE/PromptIR GenDS/00057.JPG.png} &\includegraphics[height=2.25cm, width=2.75cm]{supp_figs/Raindrop_topbox/Real/RainDS/PromptIR GenDS/14.png.png}&\includegraphics[height=2.25cm, width=2.75cm]{supp_figs/proc_supp_ood_ours/Low-light/Real/LOLv1/PromptIR GenDS/55.JPG.png}&\includegraphics[height=2.25cm, width=2.75cm]{supp_figs/proc_supp_ood_ours/Motion_blur/Real/GoPro/PromptIR GenDS/003045.png.png}&\includegraphics[height=2.25cm, width=2.75cm]{supp_figs/proc_supp_ood_ours/Rain/Real/LHP/PromptIR GenDS/10_0.png.png}&\includegraphics[height=2.25cm, width=2.75cm]{supp_figs/proc_supp_ood_ours/Snow/Synthetic/RSVD/PromptIR GenDS/0127.png.png}\\

         \rotatebox[origin=c]{90}{Swin\hspace{-56pt}}& \includegraphics[height=2.25cm, width=2.75cm]{supp_figs/proc_supp_ood_ours/Haze/Real/REVIDE/Swin/00057.JPG.png}&\includegraphics[height=2.25cm, width=2.75cm]{supp_figs/Raindrop_topbox/Real/RainDS/Swin/14.png.png}&\includegraphics[height=2.25cm, width=2.75cm]{supp_figs/proc_supp_ood_ours/Low-light/Real/LOLv1/Swin/55.JPG.png}&\includegraphics[height=2.25cm, width=2.75cm]{supp_figs/proc_supp_ood_ours/Motion_blur/Real/GoPro/Swin/003045.png.png}&\includegraphics[height=2.25cm, width=2.75cm]{supp_figs/proc_supp_ood_ours/Rain/Real/LHP/Swin/10_0.png.png}&\includegraphics[height=2.25cm, width=2.75cm]{supp_figs/proc_supp_ood_ours/Snow/Synthetic/RSVD/Swin/0127.png.png}\\

         \rotatebox[origin=c]{90}{Swin GD\hspace{-56pt}}&\includegraphics[height=2.25cm, width=2.75cm]{supp_figs/proc_supp_ood_ours/Haze/Real/REVIDE/Swin GenDS/00057.JPG.png}&\includegraphics[height=2.25cm, width=2.75cm]{supp_figs/Raindrop_topbox/Real/RainDS/Swin GenDS/14.png.png}&\includegraphics[height=2.25cm, width=2.75cm]{supp_figs/proc_supp_ood_ours/Low-light/Real/LOLv1/Swin GenDS/55.JPG.png}&\includegraphics[height=2.25cm, width=2.75cm]{supp_figs/proc_supp_ood_ours/Motion_blur/Real/GoPro/Swin GenDS/003045.png.png}&\includegraphics[height=2.25cm, width=2.75cm]{supp_figs/proc_supp_ood_ours/Rain/Real/LHP/Swin GenDS/10_0.png.png}&\includegraphics[height=2.25cm, width=2.75cm]{supp_figs/proc_supp_ood_ours/Snow/Synthetic/RSVD/Swin GenDS/0127.png.png}\\
         
         \rotatebox[origin=c]{90}{NAFNet\hspace{-56pt}}& \includegraphics[height=2.25cm, width=2.75cm]{supp_figs/proc_supp_ood_ours/Haze/Real/REVIDE/NAFNet/00057.JPG.png}&\includegraphics[height=2.25cm, width=2.75cm]{supp_figs/Raindrop_topbox/Real/RainDS/NAFNet/14.png.png}&\includegraphics[height=2.25cm, width=2.75cm]{supp_figs/proc_supp_ood_ours/Low-light/Real/LOLv1/NAFNet/55.JPG.png}&\includegraphics[height=2.25cm, width=2.75cm]{supp_figs/proc_supp_ood_ours/Motion_blur/Real/GoPro/NAFNet/003045.png.png}&\includegraphics[height=2.25cm, width=2.75cm]{supp_figs/proc_supp_ood_ours/Rain/Real/LHP/NAFNet/10_0.png.png}&\includegraphics[height=2.25cm, width=2.75cm]{supp_figs/proc_supp_ood_ours/Snow/Synthetic/RSVD/NAFNet/0127.png.png}\\

         \rotatebox[origin=c]{90}{NAFNet GD\hspace{-56pt}}& \includegraphics[height=2.25cm, width=2.75cm]{supp_figs/proc_supp_ood_ours/Haze/Real/REVIDE/NAFNet GenDS/00057.JPG.png}&\includegraphics[height=2.25cm, width=2.75cm]{supp_figs/Raindrop_topbox/Real/RainDS/NAFNet GenDS/14.png.png}&\includegraphics[height=2.25cm, width=2.75cm]{supp_figs/proc_supp_ood_ours/Low-light/Real/LOLv1/NAFNet GenDS/55.JPG.png}&\includegraphics[height=2.25cm, width=2.75cm]{supp_figs/proc_supp_ood_ours/Motion_blur/Real/GoPro/NAFNet GenDS/003045.png.png}&\includegraphics[height=2.25cm, width=2.75cm]{supp_figs/proc_supp_ood_ours/Rain/Real/LHP/NAFNet GenDS/10_0.png.png}&\includegraphics[height=2.25cm, width=2.75cm]{supp_figs/proc_supp_ood_ours/Snow/Synthetic/RSVD/NAFNet GenDS/0127.png.png}\\

         \rotatebox[origin=c]{90}{GT\hspace{-56pt}}& \includegraphics[height=2.25cm, width=2.75cm]{supp_figs/proc_supp_ood_ours/Haze/Real/REVIDE/GT/00057.JPG.png}&\includegraphics[height=2.25cm, width=2.75cm]{supp_figs/Raindrop_topbox/Real/RainDS/GT/14.png.png}&\includegraphics[height=2.25cm, width=2.75cm]{supp_figs/proc_supp_ood_ours/Low-light/Real/LOLv1/GT/55.JPG.png}&\includegraphics[height=2.25cm, width=2.75cm]{supp_figs/proc_supp_ood_ours/Motion_blur/Real/GoPro/GT/003045.png.png}&\includegraphics[height=2.25cm, width=2.75cm]{supp_figs/proc_supp_ood_ours/Rain/Real/LHP/GT/10_0.png.png}&\includegraphics[height=2.25cm, width=2.75cm]{supp_figs/proc_supp_ood_ours/Snow/Synthetic/RSVD/GT/0127.png.png}\\
    \end{tabular}
    \caption{Additional qualitative comparisons of image restoration models (PromptIR, NAFNet and the Swin model) trained  with and without our GenDS dataset. The suffix GD represents training with the GenDS dataset. Comparisons are on OoD test sets (Haze: REVIDE~\cite{revide}, Raindrop: RainDS~\cite{rainds}, Low-light: LOLv1~\cite{lolv1}, Motion blur: GoPro~\cite{gopro}, Rain: LHP~\cite{lhprain} and Snow: RSVD~\cite{rsvd}). Training with the GenDS dataset improves OoD performance. Zoomed-in patches are provided for viewing fine details.}
    \label{supfig: ood_ours}
\end{figure*}

\begin{figure*}
    \centering
    \setlength{\tabcolsep}{1pt}
    \begin{tabular}{ccccccc}
         &Haze&Raindrop&Low-light&Motion blur&Rain&Snow \\

         \rotatebox[origin=c]{90}{Input\hspace{-56pt}}&\includegraphics[height=2.25cm, width=2.75cm]{supp_figs/proc_supp_withindist_ours/Haze/Real/NH-HAZE/input/08_outdoor_GT.png.png}&\includegraphics[height=2.25cm, width=2.75cm]{supp_figs/proc_supp_withindist_ours/Raindrop/Real/Raindrop/input/19_clean.png.png}&\includegraphics[height=2.25cm, width=2.75cm]{supp_figs/proc_supp_withindist_ours/Low-light/Real/LOLv2/input/00696.png.png}&\includegraphics[height=2.25cm, width=2.75cm]{supp_figs/proc_supp_withindist_ours/Motion_blur/Real/HIDE/input/7fromGOPR0970.png.png}&\includegraphics[height=2.25cm, width=2.75cm]{supp_figs/proc_supp_withindist_ours/Rain/Synthetic/SPAC/input/00005.png.png}&\includegraphics[height=2.25cm, width=2.75cm]{supp_figs/proc_supp_withindist_ours/Snow/Synthetic/CityscapesSnow/input/berlin_000084_000019_leftimg8bit.png.png}\\

         \rotatebox[origin=c]{90}{PromptIR\hspace{-56pt}}&\includegraphics[height=2.25cm, width=2.75cm]{supp_figs/proc_supp_withindist_ours/Haze/Real/NH-HAZE/PromptIR/08_outdoor_GT.png.png}&\includegraphics[height=2.25cm, width=2.75cm]{supp_figs/proc_supp_withindist_ours/Raindrop/Real/Raindrop/PromptIR/19_clean.png.png}&\includegraphics[height=2.25cm, width=2.75cm]{supp_figs/proc_supp_withindist_ours/Low-light/Real/LOLv2/PromptIR/00696.png.png}&\includegraphics[height=2.25cm, width=2.75cm]{supp_figs/proc_supp_withindist_ours/Motion_blur/Real/HIDE/PromptIR/7fromGOPR0970.png.png}&\includegraphics[height=2.25cm, width=2.75cm]{supp_figs/proc_supp_withindist_ours/Rain/Synthetic/SPAC/PromptIR/00005.png.png}&\includegraphics[height=2.25cm, width=2.75cm]{supp_figs/proc_supp_withindist_ours/Snow/Synthetic/CityscapesSnow/PromptIR/berlin_000084_000019_leftimg8bit.png.png}\\

         \rotatebox[origin=c]{90}{PromptIR GD\hspace{-56pt}}&\includegraphics[height=2.25cm, width=2.75cm]{supp_figs/proc_supp_withindist_ours/Haze/Real/NH-HAZE/PromptIR GenDS/08_outdoor_GT.png.png}&\includegraphics[height=2.25cm, width=2.75cm]{supp_figs/proc_supp_withindist_ours/Raindrop/Real/Raindrop/PromptIR GenDS/19_clean.png.png}&\includegraphics[height=2.25cm, width=2.75cm]{supp_figs/proc_supp_withindist_ours/Low-light/Real/LOLv2/PromptIR GenDS/00696.png.png}&\includegraphics[height=2.25cm, width=2.75cm]{supp_figs/proc_supp_withindist_ours/Motion_blur/Real/HIDE/PromptIR GenDS/7fromGOPR0970.png.png}&\includegraphics[height=2.25cm, width=2.75cm]{supp_figs/proc_supp_withindist_ours/Rain/Synthetic/SPAC/PromptIR GenDS/00005.png.png}&\includegraphics[height=2.25cm, width=2.75cm]{supp_figs/proc_supp_withindist_ours/Snow/Synthetic/CityscapesSnow/PromptIR GenDS/berlin_000084_000019_leftimg8bit.png.png}\\

         \rotatebox[origin=c]{90}{Swin\hspace{-56pt}}&\includegraphics[height=2.25cm, width=2.75cm]{supp_figs/proc_supp_withindist_ours/Haze/Real/NH-HAZE/Swin/08_outdoor_GT.png.png}&\includegraphics[height=2.25cm, width=2.75cm]{supp_figs/proc_supp_withindist_ours/Raindrop/Real/Raindrop/Swin/19_clean.png.png}&\includegraphics[height=2.25cm, width=2.75cm]{supp_figs/proc_supp_withindist_ours/Low-light/Real/LOLv2/Swin/00696.png.png}&\includegraphics[height=2.25cm, width=2.75cm]{supp_figs/proc_supp_withindist_ours/Motion_blur/Real/HIDE/Swin/7fromGOPR0970.png.png}&\includegraphics[height=2.25cm, width=2.75cm]{supp_figs/proc_supp_withindist_ours/Rain/Synthetic/SPAC/Swin/00005.png.png}&\includegraphics[height=2.25cm, width=2.75cm]{supp_figs/proc_supp_withindist_ours/Snow/Synthetic/CityscapesSnow/Swin/berlin_000084_000019_leftimg8bit.png.png}\\

         \rotatebox[origin=c]{90}{Swin GD\hspace{-56pt}}&\includegraphics[height=2.25cm, width=2.75cm]{supp_figs/proc_supp_withindist_ours/Haze/Real/NH-HAZE/Swin GenDS/08_outdoor_GT.png.png}&\includegraphics[height=2.25cm, width=2.75cm]{supp_figs/proc_supp_withindist_ours/Raindrop/Real/Raindrop/Swin GenDS/19_clean.png.png}&\includegraphics[height=2.25cm, width=2.75cm]{supp_figs/proc_supp_withindist_ours/Low-light/Real/LOLv2/Swin GenDS/00696.png.png}&\includegraphics[height=2.25cm, width=2.75cm]{supp_figs/proc_supp_withindist_ours/Motion_blur/Real/HIDE/Swin GenDS/7fromGOPR0970.png.png}&\includegraphics[height=2.25cm, width=2.75cm]{supp_figs/proc_supp_withindist_ours/Rain/Synthetic/SPAC/Swin GenDS/00005.png.png}&\includegraphics[height=2.25cm, width=2.75cm]{supp_figs/proc_supp_withindist_ours/Snow/Synthetic/CityscapesSnow/Swin GenDS/berlin_000084_000019_leftimg8bit.png.png}\\
         
         \rotatebox[origin=c]{90}{NAFNet\hspace{-56pt}}&\includegraphics[height=2.25cm, width=2.75cm]{supp_figs/proc_supp_withindist_ours/Haze/Real/NH-HAZE/NAFNet/08_outdoor_GT.png.png}&\includegraphics[height=2.25cm, width=2.75cm]{supp_figs/proc_supp_withindist_ours/Raindrop/Real/Raindrop/NAFNet/19_clean.png.png}&\includegraphics[height=2.25cm, width=2.75cm]{supp_figs/proc_supp_withindist_ours/Low-light/Real/LOLv2/NAFNet/00696.png.png}&\includegraphics[height=2.25cm, width=2.75cm]{supp_figs/proc_supp_withindist_ours/Motion_blur/Real/HIDE/NAFNet/7fromGOPR0970.png.png}&\includegraphics[height=2.25cm, width=2.75cm]{supp_figs/proc_supp_withindist_ours/Rain/Synthetic/SPAC/NAFNet/00005.png.png}&\includegraphics[height=2.25cm, width=2.75cm]{supp_figs/proc_supp_withindist_ours/Snow/Synthetic/CityscapesSnow/NAFNet/berlin_000084_000019_leftimg8bit.png.png}\\

         \rotatebox[origin=c]{90}{NAFNet GD\hspace{-56pt}}&\includegraphics[height=2.25cm, width=2.75cm]{supp_figs/proc_supp_withindist_ours/Haze/Real/NH-HAZE/NAFNet GenDS/08_outdoor_GT.png.png}&\includegraphics[height=2.25cm, width=2.75cm]{supp_figs/proc_supp_withindist_ours/Raindrop/Real/Raindrop/NAFNet GenDS/19_clean.png.png}&\includegraphics[height=2.25cm, width=2.75cm]{supp_figs/proc_supp_withindist_ours/Low-light/Real/LOLv2/NAFNet GenDS/00696.png.png}&\includegraphics[height=2.25cm, width=2.75cm]{supp_figs/proc_supp_withindist_ours/Motion_blur/Real/HIDE/NAFNet GenDS/7fromGOPR0970.png.png}&\includegraphics[height=2.25cm, width=2.75cm]{supp_figs/proc_supp_withindist_ours/Rain/Synthetic/SPAC/NAFNet GenDS/00005.png.png}&\includegraphics[height=2.25cm, width=2.75cm]{supp_figs/proc_supp_withindist_ours/Snow/Synthetic/CityscapesSnow/NAFNet GenDS/berlin_000084_000019_leftimg8bit.png.png}\\

         \rotatebox[origin=c]{90}{GT\hspace{-56pt}}&\includegraphics[height=2.25cm, width=2.75cm]{supp_figs/proc_supp_withindist_ours/Haze/Real/NH-HAZE/GT/08_outdoor_GT.png.png}&\includegraphics[height=2.25cm, width=2.75cm]{supp_figs/proc_supp_withindist_ours/Raindrop/Real/Raindrop/GT/19_clean.png.png}&\includegraphics[height=2.25cm, width=2.75cm]{supp_figs/proc_supp_withindist_ours/Low-light/Real/LOLv2/GT/00696.png.png}&\includegraphics[height=2.25cm, width=2.75cm]{supp_figs/proc_supp_withindist_ours/Motion_blur/Real/HIDE/GT/7fromGOPR0970.png.png}&\includegraphics[height=2.25cm, width=2.75cm]{supp_figs/proc_supp_withindist_ours/Rain/Synthetic/SPAC/GT/00005.png.png}&\includegraphics[height=2.25cm, width=2.75cm]{supp_figs/proc_supp_withindist_ours/Snow/Synthetic/CityscapesSnow/GT/berlin_000084_000019_leftimg8bit.png.png}\\
    \end{tabular}
    \caption{Qualitative comparisons of image restoration models on within-distribution test sets when trained with and without our GenDS dataset. The suffix GD represents training with the GenDS dataset. Images are from the following test sets - Haze: NH-Haze~\cite{nhhaze}, Raindrop: Raindrop~\cite{raindrop}, Low-light: LOLv2~\cite{lolv2}, Motion blur: HIDE~\cite{hide} and Snow: SnowyCityscapes~\cite{snowcity}. Zoomed-in patches are provided for viewing fine details.}
    \label{supfig: within_dist_ours}
\end{figure*}

\begin{figure*}
    \centering
    \setlength{\tabcolsep}{1pt}
    \begin{tabular}{cccccc}
         &Haze&Low-light&Rain&Motion blur\\

         \rotatebox[origin=c]{90}{Input\hspace{-56pt}}&\includegraphics[height=2.15cm, width=2.75cm]{supp_figs/proc_supp_ood_others/Haze/Real/O-HAZE/input/21_outdoor_GT.png.png}&\includegraphics[height=2.15cm, width=2.75cm]{supp_figs/proc_supp_ood_others/Low-light/Real/SICE/input/55_2.JPG.png}&\includegraphics[height=2.15cm, width=2.75cm]{supp_figs/proc_supp_ood_others/Rain/Real/LHP/input/12_1.png.png}&\includegraphics[height=2.15cm, width=2.75cm]{supp_figs/proc_supp_ood_others/Motion_blur/Real/GoPro/input/004090.png.png}\\

         \rotatebox[origin=c]{90}{DiffUIR\hspace{-56pt}}&\includegraphics[height=2.15cm, width=2.75cm]{supp_figs/proc_supp_ood_others/Haze/Real/O-HAZE/diffuir/21_outdoor_GT.png.png}&\includegraphics[height=2.15cm, width=2.75cm]{supp_figs/proc_supp_ood_others/Low-light/Real/SICE/diffuir/55_2.JPG.png}&\includegraphics[height=2.15cm, width=2.75cm]{supp_figs/proc_supp_ood_others/Rain/Real/LHP/diffuir/12_1.png.png}&\includegraphics[height=2.15cm, width=2.75cm]{supp_figs/proc_supp_ood_others/Motion_blur/Real/GoPro/diffuir/004090.png.png}\\

         \rotatebox[origin=c]{90}{Diff-Plugin\hspace{-56pt}}&\includegraphics[height=2.15cm, width=2.75cm]{supp_figs/proc_supp_ood_others/Haze/Real/O-HAZE/diffplugin/21_outdoor_GT.png.png}&\includegraphics[height=2.15cm, width=2.75cm]{supp_figs/proc_supp_ood_others/Low-light/Real/SICE/diffplugin/55_2.JPG.png}&\includegraphics[height=2.15cm, width=2.75cm]{supp_figs/proc_supp_ood_others/Rain/Real/LHP/diffplugin/12_1.png.png}&\includegraphics[height=2.15cm, width=2.75cm]{supp_figs/proc_supp_ood_others/Motion_blur/Real/GoPro/diffplugin/004090.png.png}\\

         \rotatebox[origin=c]{90}{InstructIR\hspace{-56pt}}&\includegraphics[height=2.15cm, width=2.75cm]{supp_figs/proc_supp_ood_others/Haze/Real/O-HAZE/instructir/21_outdoor_GT.png.png}&\includegraphics[height=2.15cm, width=2.75cm]{supp_figs/proc_supp_ood_others/Low-light/Real/SICE/instructir/55_2.JPG.png}&\includegraphics[height=2.15cm, width=2.75cm]{supp_figs/proc_supp_ood_others/Rain/Real/LHP/instructir/12_1.png.png}&\includegraphics[height=2.15cm, width=2.75cm]{supp_figs/proc_supp_ood_others/Motion_blur/Real/GoPro/instructir/004090.png.png}\\

         \rotatebox[origin=c]{90}{AutoDIR\hspace{-56pt}}&\includegraphics[height=2.15cm, width=2.75cm]{supp_figs/proc_supp_ood_others/Haze/Real/O-HAZE/autodir/21_outdoor_GT.png.png}&\includegraphics[height=2.15cm, width=2.75cm]{supp_figs/proc_supp_ood_others/Low-light/Real/SICE/autodir/55_2.JPG.png}&\includegraphics[height=2.15cm, width=2.75cm]{supp_figs/proc_supp_ood_others/Rain/Real/LHP/autodir/12_1.png.png}&\includegraphics[height=2.15cm, width=2.75cm]{supp_figs/proc_supp_ood_others/Motion_blur/Real/GoPro/autodir/004090.png.png}\\
         
         \rotatebox[origin=c]{90}{PromptIR GD\hspace{-56pt}}&\includegraphics[height=2.15cm, width=2.75cm]{supp_figs/proc_supp_ood_others/Haze/Real/O-HAZE/PromptIR GenDS/21_outdoor_GT.png.png}&\includegraphics[height=2.15cm, width=2.75cm]{supp_figs/proc_supp_ood_others/Low-light/Real/SICE/PromptIR GenDS/55_2.JPG.png}&\includegraphics[height=2.15cm, width=2.75cm]{supp_figs/proc_supp_ood_others/Rain/Real/LHP/PromptIR GenDS/12_1.png.png}&\includegraphics[height=2.15cm, width=2.75cm]{supp_figs/proc_supp_ood_others/Motion_blur/Real/GoPro/PromptIR GenDS/004090.png.png}\\

         \rotatebox[origin=c]{90}{Swin GD\hspace{-56pt}}&\includegraphics[height=2.15cm, width=2.75cm]{supp_figs/proc_supp_ood_others/Haze/Real/O-HAZE/Swin GenDS/21_outdoor_GT.png.png}&\includegraphics[height=2.15cm, width=2.75cm]{supp_figs/proc_supp_ood_others/Low-light/Real/SICE/Swin GenDS/55_2.JPG.png}&\includegraphics[height=2.15cm, width=2.75cm]{supp_figs/proc_supp_ood_others/Rain/Real/LHP/Swin GenDS/12_1.png.png}&\includegraphics[height=2.15cm, width=2.75cm]{supp_figs/proc_supp_ood_others/Motion_blur/Real/GoPro/Swin GenDS/004090.png.png}\\

         \rotatebox[origin=c]{90}{NAFNet GD\hspace{-56pt}}&\includegraphics[height=2.15cm, width=2.75cm]{supp_figs/proc_supp_ood_others/Haze/Real/O-HAZE/NAFNet GenDS/21_outdoor_GT.png.png}&\includegraphics[height=2.15cm, width=2.75cm]{supp_figs/proc_supp_ood_others/Low-light/Real/SICE/NAFNet GenDS/55_2.JPG.png}&\includegraphics[height=2.15cm, width=2.75cm]{supp_figs/proc_supp_ood_others/Rain/Real/LHP/NAFNet GenDS/12_1.png.png}&\includegraphics[height=2.15cm, width=2.75cm]{supp_figs/proc_supp_ood_others/Motion_blur/Real/GoPro/NAFNet GenDS/004090.png.png}\\

         \rotatebox[origin=c]{90}{GT\hspace{-56pt}}&\includegraphics[height=2.15cm, width=2.75cm]{supp_figs/proc_supp_ood_others/Haze/Real/O-HAZE/GT/21_outdoor_GT.png.png}&\includegraphics[height=2.15cm, width=2.75cm]{supp_figs/proc_supp_ood_others/Low-light/Real/SICE/GT/55_2.JPG.png}&\includegraphics[height=2.15cm, width=2.75cm]{supp_figs/proc_supp_ood_others/Rain/Real/LHP/GT/12_1.png.png}&\includegraphics[height=2.15cm, width=2.75cm]{supp_figs/proc_supp_ood_others/Motion_blur/Real/GoPro/GT/004090.png.png}
    \end{tabular}
    \caption{Qualitative comparisons for OoD performance of image restoration models (PromptIR, NAFNet and the Swin model) trained with our GenDS dataset, and SOTA AIOR approaches, namely, DiffUIR~\cite{diffuir}, Diff-Plugin~\cite{diffplugin}, InstructIR~\cite{instructir} and AutoDIR~\cite{autodir}. Images are from the following datasets- Haze: O-Haze~\cite{ohaze}, Low-light: SICE~\cite{sice}, Rain: LHP~\cite{lhprain} and Motion Blur: Go Pro~\cite{gopro}.}
    \label{supfig:ood_others}
\end{figure*}

\begin{figure*}
    \centering
    \setlength{\tabcolsep}{1pt}
    \begin{tabular}{ccccccc}
        Input&DiffUIR&Diff-Plugin&PromptIR GD&Swin GD&NAFNet GD&GT\\
        
        \includegraphics[height=2.25cm, width=2.45cm]{supp_figs/proc_supp_ood_others/Snow/Synthetic/RSVD/input/0159.png.png}&\includegraphics[height=2.25cm, width=2.45cm]{supp_figs/proc_supp_ood_others/Snow/Synthetic/RSVD/diffuir/0159.png.png}&\includegraphics[height=2.25cm, width=2.45cm]{supp_figs/proc_supp_ood_others/Snow/Synthetic/RSVD/diffplugin/0159.png.png}&\includegraphics[height=2.25cm, width=2.45cm]{supp_figs/proc_supp_ood_others/Snow/Synthetic/RSVD/PromptIR GenDS/0159.png.png}&\includegraphics[height=2.25cm, width=2.45cm]{supp_figs/proc_supp_ood_others/Snow/Synthetic/RSVD/Swin GenDS/0159.png.png}&\includegraphics[height=2.25cm, width=2.45cm]{supp_figs/proc_supp_ood_others/Snow/Synthetic/RSVD/NAFNet GenDS/0159.png.png}&\includegraphics[height=2.25cm, width=2.4cm]{supp_figs/proc_supp_ood_others/Snow/Synthetic/RSVD/GT/0159.png.png}
    \end{tabular}
    \caption{Qualitative comparisons of OoD performance of image restoration models (PromptIR, NAFNet and the Swin model) trained with our GenDS dataset, and SOTA AIOR approaches, namely, DiffUIR~\cite{diffuir}, Diff-Plugin~\cite{diffplugin} for the task of desnowing on the RSVD~\cite{rsvd} dataset.}
    \label{supfig:ood_others_snow}
\end{figure*}

\begin{figure*}
    \centering
    \setlength{\tabcolsep}{1pt}
    \begin{tabular}{cccccc}
        Input&AutoDIR&PromptIR GD&Swin GD&NAFNet GD&GT\\
        
        \includegraphics[height=2.25cm, width=2.75cm]{supp_figs/proc_supp_ood_others/Raindrop/Real/RainDS/input/64.png.png}&\includegraphics[height=2.25cm, width=2.75cm]{supp_figs/proc_supp_ood_others/Raindrop/Real/RainDS/autodir/64.png.png}&\includegraphics[height=2.25cm, width=2.75cm]{supp_figs/proc_supp_ood_others/Raindrop/Real/RainDS/PromptIR GenDS/64.png.png}&\includegraphics[height=2.25cm, width=2.75cm]{supp_figs/proc_supp_ood_others/Raindrop/Real/RainDS/Swin GenDS/64.png.png}&\includegraphics[height=2.25cm, width=2.75cm]{supp_figs/proc_supp_ood_others/Raindrop/Real/RainDS/NAFNet GenDS/64.png.png}&\includegraphics[height=2.25cm, width=2.75cm]{supp_figs/proc_supp_ood_others/Raindrop/Real/RainDS/GT/64.png.png}
    \end{tabular}
    \caption{Qualitative comparisons for OoD performance of image restoration models (PromptIR, NAFNet and the Swin model) trained with our GenDS dataset, and AutoDIR, a SOTA AIOR approach, for the task of raindrop removal on the RainDS~\cite{rainds} dataset.}
    \label{supfig:ood_others_raindrop}
\end{figure*}
